# Supplementary material for: Dynamical Boundary Following and Corner Trapping of Undulating Worms
Source: arXiv:2501.10783 source file (2026-02-15)
Supplement: Supplementary file 1 [file SI.pdf]

# Supplementary Materials

## Boundary curvature-dependent dynamical trapping of undulating worms

Sohum Kapadia and Arshad Kudrolli  
*Department of Physics, Clark University, Worcester, MA 01610*  
(Dated: January 8, 2025)

### I. MOVIES

List of movies and captions.

- Movie S1: A California blackworm moving in a circular chamber is observed to turn and follow the boundary. The frame rate is 1 fps and total time is 450 s. ( $R = 20$  mm;  $l_w = 18 \pm 1.50$  mm). The movie is played at 10 fps.
- Movie S2: A California blackworm moving in a square chamber is observed to turn and follow the boundary and get trapped at the corners before escaping over varying internal of time. The frame rate is 1 fps and total time is 600 s. ( $l = 40$  mm;  $l_w = 22 \pm 2$  mm). The movie is played at 10 fps.
- Movie S3: A California blackworm moving in a polygonal chamber with concave and convex corners. The worm is observed to follow the boundary but not round convex corners. It is observed to get trapped at concave corners as also seen in the square chambers. The frame rate is 1 fps and total time is 600 s. ( $l = 40$  mm;  $l_w = 15 \pm 1.8$  mm). The movie is played at 10 fps.
- Movie S4: An animation of simulated dumbbell model in a circular chamber. The frame rate is 4 fps and total time is 180 s. The animation is played at frame rate of 40 fps.
- Movie S5: An animation of simulated dumbbell model in a square chamber. The frame rate is 4 fps and total time is 600 s. The animation is played at frame rate of 40 fps.
- Movie S6: An animation of simulated dumbbell model in a polygon chamber. The frame rate is 4 fps and total time is 600 s. The animation is played at frame rate of 40 fps.

### II. IMAGE PROCESSING

The system is imaged from top with a DSLR camera Canon Rebel T5i while the worms are back-lit with a uniform LED array. After the worms acclimatize over a few minutes, the motion of the worm is recorded for about 30 minutes at 24 fps, and the worm is returned back to the holding tank. A representative image is shown in Fig. 1(a). The images are binarized by using a suitable threshold and its complementary is shown in Fig. 1(b) and the entire shape of the worm is tracked using Image Acquisition Toolbox functions implemented in MATLAB. The tracked worm body position superimposed on an image of the worm is shown in Fig. 1(c), and several superimposed snapshots of the worm while moving inside the chamber is shown in Fig. 1(d). We obtain the worm locomotion speed, its orientation, the stroke amplitudes, along with the position of the head and tail from the tracked shape, and use them for further analysis.

The recorded images are pre-processed before they can be used for extracting data. We use the following steps for pre-processing:

1. **Conversion of an image from RGB to gray scale.** The image captured by the camera is in RGB scale. We convert the image to gray scale. In images obtained using above mentioned lighting, worm appears dark in contrast to bright background.
2. **Subtracting the background from the image.** To remove the background, we average over all the images to obtain the background image. Then we subtract the image from the background image. The resulting complementary image has bright pixels corresponding to worm body and dark background.
3. **Binarizing the image.** The gray scale images are binarized using an appropriate threshold. We set the threshold value such that the worm's body pixel value is equal to 1.
4. **Cleaning the image.** The noise in the binarized image is removed by determining all the connected objects in the image and choosing the object having maximum number of pixels which corresponds to worm body.

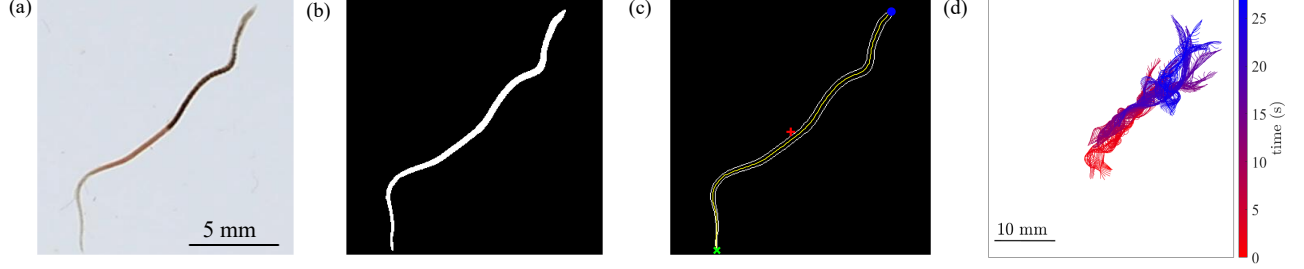

FIG. 1. (a) A closeup image of a California blackworm. (b) The complementary binarized image. (c) Tracked body shape (solid yellow curve) of the worm with head (blue o), centroid (red +) and tail (green x) coordinates. (d) Superimposed snapshots of a worm moving diagonally across a square chamber at 12 frames per second or 83.3 ms time intervals. The color bar represents time.

**5. Skeletonizing the image.** We then determine the skeleton of the image. The skeleton image is a 2D curved line representing the body shape of the worm.

The position coordinates for the head, centroid and tail of the worm can be tracked from the processed image. Using inbuilt MATLAB operations we can directly extract the position of the centroid of any segment (here the worm body) present in the image. To track head and tail, we extract and save the endpoints from the images and connect them using the Hungarian tracking algorithm. To track the full body shape of the worm we use the skeleton image and sort its pixel from head to tail using the tracked head and tail coordinates.

### III. BOUNDARY ALIGNING DYNAMICS IN CIRCULAR CHAMBER

A typical trajectory of a worm of length  $l_w = 28 \pm 2.3$  mm moving in the circular chamber with radius  $R = 20$  mm is shown in Fig. 2(a) over time  $T = 375$  s (Movie S7). Plotting the histogram of its centroid in Fig. 2(b) we observe that it stays approximately at a distance of  $3R/4$  from the center. This occurs because the worm is observed to maintain a more or less constant body angle with respect to the normal to the boundary.

We further show in Fig. 2(c) the trajectory obtained with active elastic dumbbell model and observe similar boundary following behavior. The choice of  $Pe$  is found to affect of the degree to which the centroid distance fluctuates from the center. The Probability distribution of the centroid position observed in simulations shown in Fig. 2(d) are observed to be similar to those in the experiments.

Using the kinematic rod model for boundary alignment in a circular chamber we can determine the equilibrium orientation of the worm with respect to the normal.

$$\frac{d\theta}{dt} = \sin(2\theta) - \frac{l}{R} \sin(\theta), \text{ and} \quad (1)$$

$$\theta_o = \cos^{-1} \left( \frac{l}{2R} \right). \quad (2)$$

Here,  $l$  is the length of the rod and  $R$  is the radius of the circular chamber,  $\theta$  is angle between the rod and the normal to the boundary.

### IV. LOCOMOTION SPEED OF THE WORMS

We determine the speed of the worms while they are away from the boundary, close to the boundary or at a corner. In order to do so, we consider all the corresponding events from 10 trials each performed for 30 minutes. The average speed is calculated from the coordinates at a chosen time interval. The time interval is set equal to an integral multiple of the time period of a peristaltic stroke,  $T = 2.5$  seconds.

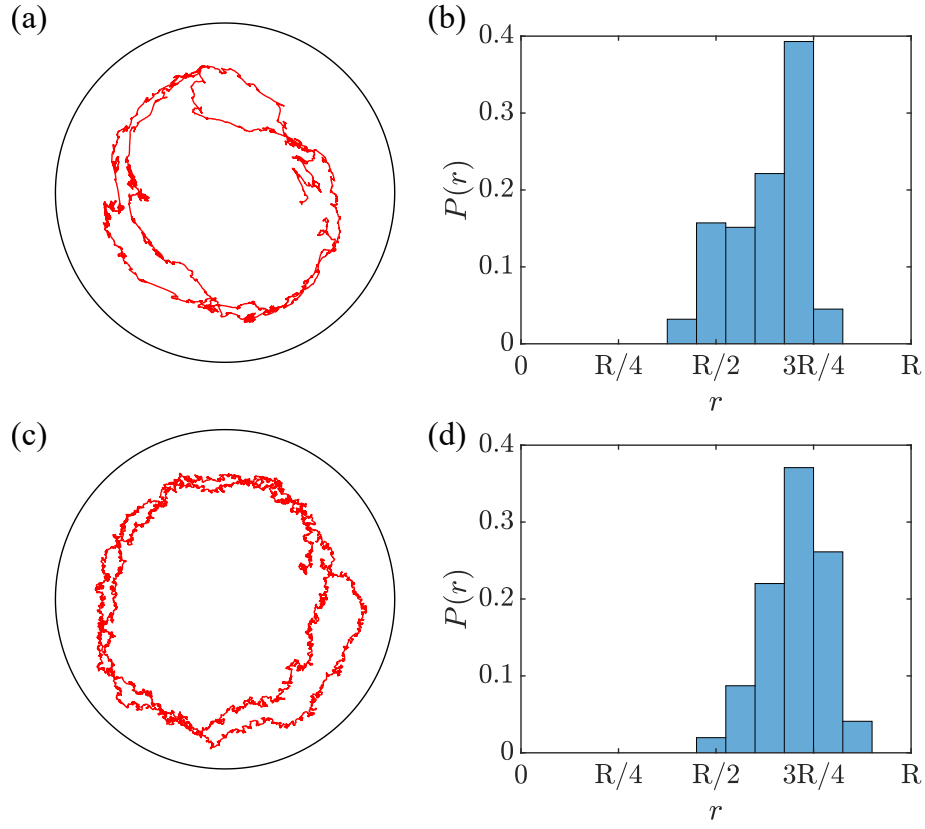

FIG. 2. (a) The trajectory of a worm centroid in a circular chamber over time  $T = 375$  seconds. (b) PDF of centroid distance from the circle center. The angle that the worm's body makes with the normal to surface  $\psi_b \approx 65^\circ$ . (c,d) Corresponding active dumbbell simulated centroid trajectory and distribution for  $\alpha_p = 2$  and  $\epsilon = 4 \times 10^4$  to roughly match the speed and the centroid distribution width of the dumbbell, respectively so that  $Pe = 5 \times 10^{-3}$ .

Centroid speed:

$$\begin{aligned} \text{Away from boundary, } v_c &= 0.95 \pm 0.49 \text{ mm s}^{-1} \\ \text{Near boundary, } v_c &= 0.82 \pm 0.57 \text{ mm s}^{-1} \\ \text{Near Corner, } v_c &= 0.47 \pm 0.15 \text{ mm s}^{-1} \end{aligned}$$

Head speed:

$$\begin{aligned} \text{Away from boundary, } v_h &= 1.72 \pm 0.65 \text{ mm s}^{-1} \\ \text{Near boundary, } v_h &= 1.33 \pm 0.70 \text{ mm s}^{-1} \\ \text{Near Corner, } v_h &= 0.26 \pm 0.07 \text{ mm s}^{-1} \end{aligned}$$

Thus, we observe that the velocity of both the centroid and the head while confined in the corner is significantly lower than when it is away from the boundaries due to the inelastic collisions with the boundaries. Further, it can be noted from the speeds that the head is more motile than the centroid in each region, except in the concave corner.

|               | Centre | Boundary | Corner |
|---------------|--------|----------|--------|
| $T_L$ (in s)  | 1.83   | 1.46     | 1.33   |
| $A_L$ (in mm) | 1.90   | 3.23     | 1.30   |
| $T_T$ (in s)  | 9.17   | 1.46     | 11.08  |
| $A_T$ (in mm) | 1.34   | 1.00     | 2.18   |

TABLE I. Transverse and Longitudinal stroke amplitude while in center, boundary and corner region of the chamber.

## V. PERISTALTIC AND UNDULATORY STROKES

We determine the frequency and amplitude for the transverse/longitudinal strokes performed by *L. variegatus* in a water filled square chamber. We further contrast this values based on the worm location at the center, boundary or corner region in the chamber.

### Peristaltic strokes

The body length of the worm oscillates owing to the peristaltic strokes performed by the worm as shown in Fig. 3(a). We assume the motion to be 2D and neglect any length variation due to out of plane motion of worm body. To characterize its frequency and amplitude, we calculate the length correlation function as shown in Fig. 3(b),

$$K_L(t) = \langle \Delta l_w(t + t_o) \Delta l_w(t) \rangle / \langle \Delta l_w^2 \rangle.$$

Here,  $\Delta l_w$  denotes the variation of the worm length from its mean length. The mean squared length variation,  $\langle \Delta l_w^2 \rangle$  is computed over time interval  $T_L$ . The first peak in the length correlation function can be associated to the time period of the peristaltic stroke  $T_L$  as pointed by the black arrow in Fig. 3(b). The amplitude  $A_L$  can be determined using the magnitude of the first peak which is equal to  $A_L^2 / (2 \langle \Delta l_w^2 \rangle)$ . The magnitude of  $A_L$  for each region is mentioned in Table I. We observe that the time period of the peristalsis strokes is about  $T_L \approx 1.5$  s independent of the location of the worm. while worm is near a boundary it performs peristalsis strokes with largest amplitude of  $A_L = 3$  mm.

Further we calculate the velocity correlation function,

$$K_v(t) = \langle v_w(t + t_o) v_w(t) \rangle / v_w^2,$$

where  $v_w(t)$  is the worm head speed at time  $t$ ,  $v_w = 1.38$  mm s<sup>-1</sup> is the worm head speed, calculated over a time interval of 10 s while worm is moving across the chamber away from the boundary. In Fig 3(c), the peaks of velocity correlation occurs at the same time periods  $T_l$  as the length correlation.

### Undulatory strokes

We calculate the transverse stroke amplitude using the root mean squared displacement in the body frame of reference  $A_T = \sqrt{\langle y^2 \rangle}$ , averaged over its length. The magnitudes of transverse amplitude are mentioned in Table I. To determine the undulatory strokes time period  $T_T$ , we show transverse amplitude correlation,

$$K_T(t) = \langle y_c(t + t_o) y_c(t) \rangle / \langle y_c^2 \rangle,$$

where  $y_c$  is the displacement of the midsection of the worm body from body axis. In Fig 3(d) we observe a peak at  $T_T$ .

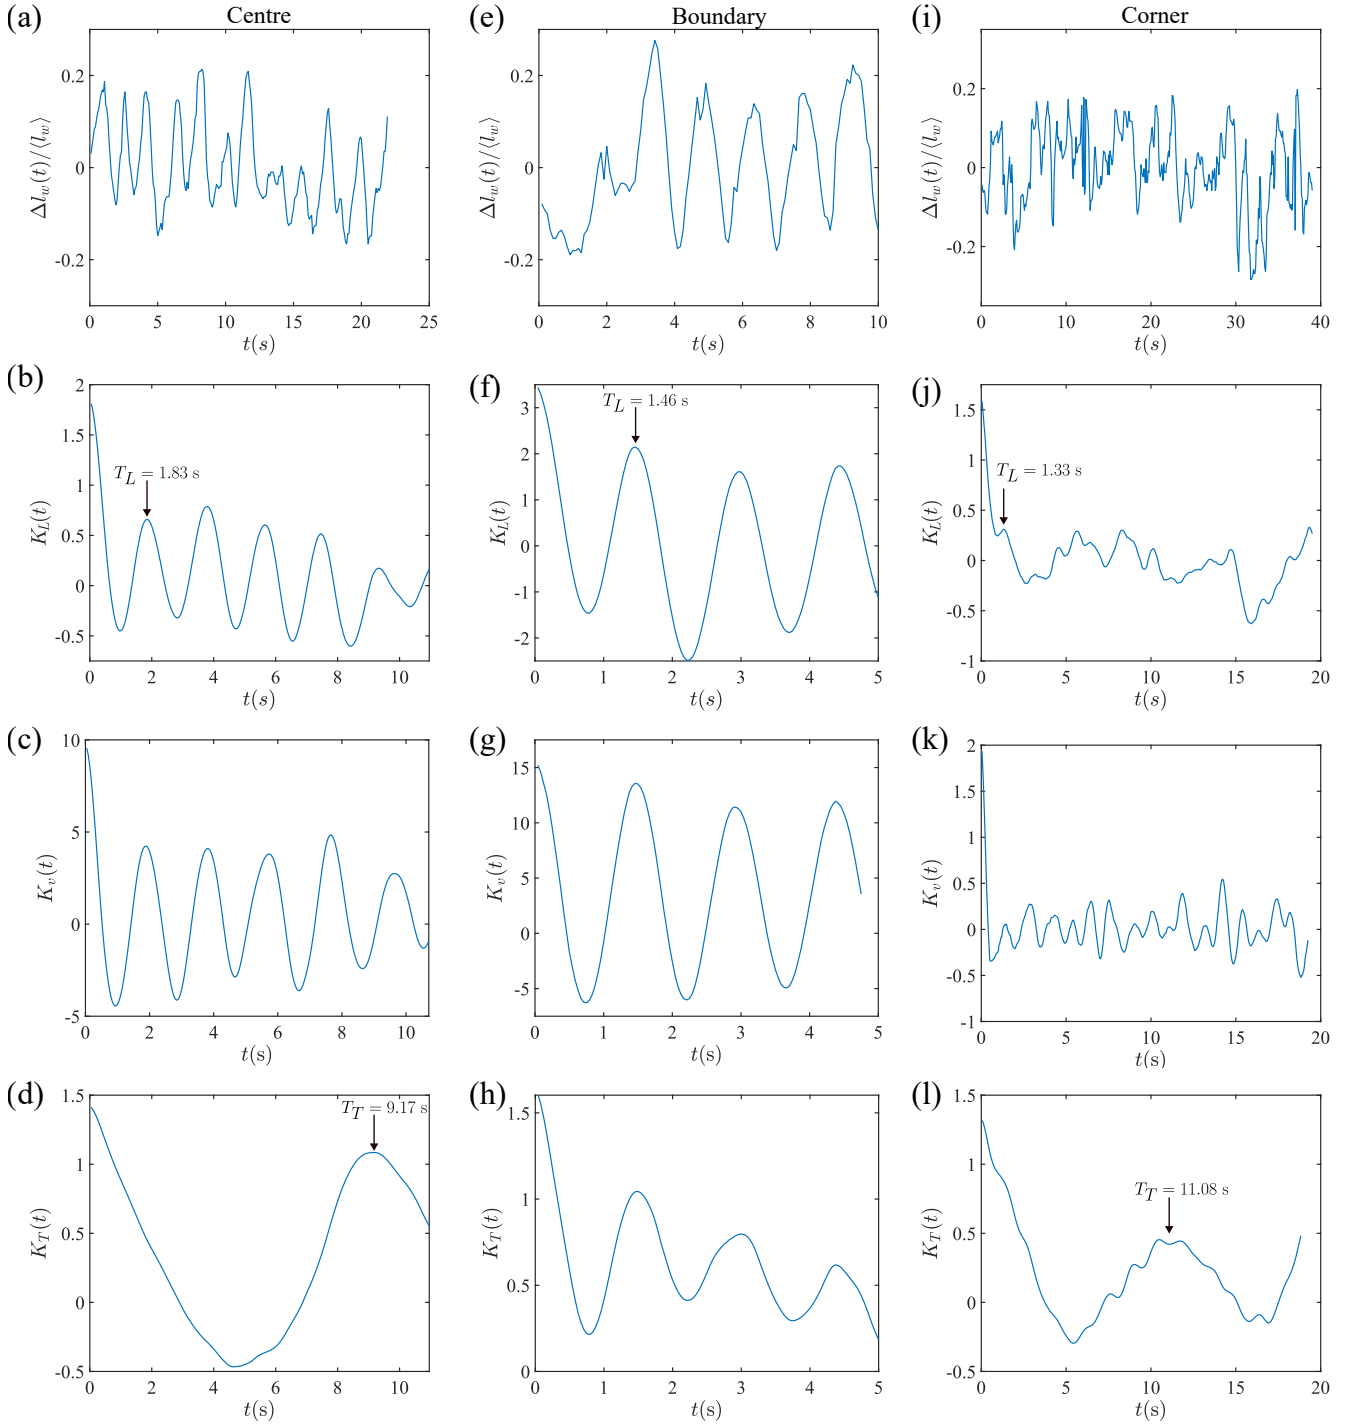

FIG. 3. The length oscillations and correlation functions corresponding to center, boundary and corner regions. While the leading peaks in  $K_L$  and  $K_v$  are coordinated while the worm moves forward in the central and boundary regions, the peaks are absent while the worm is stuck in the corners as it does not move forward.
